# Supplementary material for: First-Order vs. Second-Order Encodings for LTLf-to-Automata Translation
Source: arXiv:1901.06108 source file (2019-01-18)
Supplement: Supplementary file 1 [file Appendix.tex]

\newpage
\appendix
To make the paper self-contained, we now show the proofs omitted from the body of the paper due to page limit.
\section{\MSO Encoding}\label{app:mso}
The section gives the proofs of the \MSO encoding and various variations described in Section~\ref{sec:mso}.
\subsection{\LTLf to \MSO Encoding}
The following theorem guarantees the correctness of \MSO encoding.
\begin{thm}
Let $\phi$ be an \LTLf formula, $\rho$ be a finite trace. Then $\rho \models \phi$ iff $\I_\rho\models \mathsf{mso}(\phi)$.
\end{thm}
\begin{proof}

If $\phi$ is a propositional atom $p$, then $\mathsf{mso}(\phi)=Q_p(0)$. It is true that $\rho \models \phi$ iff $\I_\rho \models \mathsf{mso}(\phi)$. If $\phi$ is an nonatomic formula, we prove this theorem in two directions.

Suppose first that $\rho$ satisfies $\phi$. We expand the monadic structure $\I_\rho$ with interpretations for the existentially quantified monadic predicate symbols by setting $Q^\I_{\theta_i}$ as the set collecting all points of $\rho$ satisfying $\theta_i$, that is $Q^\I_{\theta_i}=\{x~:~\rho,x\models\theta_i\}$. We also define $Q_p=\{x~:~\rho,x\models p\}$. Denote the expanded structure by $\I_\rho^{mso}$. By assumption, $Q_\phi(0)$ holds in $\I_\rho^{mso}$.
It remains to prove that $\I_\rho^{mso}\models \forall x.\mathsf{t}(\theta_i,x)$, for each nonatomic subformula $\theta_i\in cl(\phi)$, which we prove via structural induction over $\theta_i$.
\begin{itemize}
% \item 
% Claim holds trivially for atomic formulas.
\item 
If $\theta_i =(\neg \theta_j$), then $\mathsf{t}(\theta_i,x) = (Q_{\theta_i}(x) \leftrightarrow (x \notin Q_{\theta_j}))$. This holds, since $Q_{(\neg\theta_j)}^\I=\{x~:~\rho,x\not\models\theta_j\}$ and $Q_{\theta_j}^\I=\{x~:~\rho,x\models\theta_j\}$.
\item
If $\theta_i = (\theta_j \wedge \theta_k)$, then $\mathsf{t}(\theta_i,x) = (Q_{\theta_i}(x) \leftrightarrow (Q_{\theta_j}(x) \wedge Q_{\theta_k}(x)))$. This holds, since $Q_{(\theta_j\wedge\theta_k)}^\I=\{x~:~\rho,x\models\theta_j\mbox{ and }\rho,x\models\theta_k\}$, $Q_{\theta_j}^\I=\{x~:~\rho,x\models\theta_j\}$ and $Q_{\theta_k}^\I=\{x~:~\rho,x\models\theta_k\}$.
\item
If $\theta_i = (\theta_j \vee \theta_k)$, then $\mathsf{t}(\theta_i,x) = (Q_{\theta_i}(x) \leftrightarrow (Q_{\theta_j}(x) \vee Q_{\theta_k}(x)))$. This holds, since $Q_{(\theta_j\vee\theta_k)}^\I=\{x~:~\rho,x\models\theta_j\mbox{ or }\rho,x\models\theta_k\}$, $Q_{\theta_j}^\I=\{x~:~\rho,x\models\theta_j\}$ and $Q_{\theta_k}^\I=\{x~:~\rho,x\models\theta_k\}$.
\item
If $\theta_i = (X\theta_j)$, then $\mathsf{t}(\theta_i,x) = (Q_{\theta_i}(x)\leftrightarrow ((x \neq last)\wedge Q_{\theta_j}(x+1)))$.
This holds, since $Q_{(X\theta_i)}^\I=\{x~:~\rho,x\models (X\theta_j)\}=\{x~:~ x \neq last\mbox{ and } \rho,x+1\models\theta_j\}$, and $Q_{\theta_j}=\{x~:~\rho,x\models\theta_j\}$.
\item
If $\theta_i = (N\theta_j)$, then $\mathsf{t}(\theta_i,x) = (Q_{\theta_i}(x)\leftrightarrow ((x = last)\vee Q_{\theta_j}(x+1)))$. This holds, since $Q_{(N\theta_i)}^\I=\{x~:~\rho,x\models (N\theta_j)\}=\{x~:~ x=last\mbox{ or } \rho,x+1\models\theta_j\}$, and $Q_{\theta_j}=\{x~:~\rho,x\models\theta_j\}$.

\item If $\theta_i = (\theta_j U \theta_k)$, then $\mathsf{t}(\theta_i,x) = (Q_{\theta_i}(x) \leftrightarrow (Q_{\theta_k}(x) \vee ((x \neq last) \wedge Q_{\theta_j}(x) \wedge Q_{\theta_i}(x+1))))$. This holds, since $Q_{(\theta_j U \theta_k)}^{\mathcal{I}} = \{x~:~\rho,x \models \theta_j U \theta_k\} = \{x~:~\rho,x \models \theta_k \mbox{ or } x \neq last \mbox{ with } \rho,x \models \theta_j \mbox{ also } \rho,x+1 \models \theta_i \}$, $Q_{\theta_j} = \{x~:~\rho,x \models \theta_j\}$, and $Q_{\theta_k} = \{x~:~\rho,x \models \theta_k\}$;

\item If $\theta_i = (\theta_j R \theta_k)$, then $\mathsf{t}(\theta_i,x) = (Q_{\phi}(x) \leftrightarrow (Q_{\theta_k}(x) \wedge ((x = last) \vee Q_{\theta_j}(x) \vee Q_{\theta_i}(x+1))))$. This holds, since $Q_{(\theta_j R \theta_k)}^{\mathcal{I}} = \{x~:~\rho,x \models \theta_j R \theta_k\} = \{x~:~\rho,x \models \theta_k \mbox{ with } x = last \mbox{ or } \rho,x \models \theta_j \mbox{ or } \rho,x+1 \models \theta_i \}$, $Q_{\theta_j} = \{x~:~\rho,x \models \theta_j\}$, and $Q_{\theta_k} = \{x~:~\rho,x \models \theta_k\}$.
\end{itemize}
%With above, it has been proven that $\mathcal{I}_{\rho}^{mso} \models mso(\phi)$; 

Assume now that $\I_\rho\models \mathsf{mso}(\phi)$. This means that there is an 
expansion of $\I_\rho$ with monadic interpretations $Q_{\theta_i}^\I$ for each nonatomic subformula $\theta_i\in cl(\phi)$ such that this expanded structure $\I_\rho^{mso}\models (Q_\phi(0)\wedge ((\forall x)\bigwedge_{i=1}^{m}\mathsf{t}(\theta_i,x)))$. We now prove by induction on $\phi$ that if $x\in Q_{\theta_i}^\I$, then $\rho,x\models\theta_i$. Since $\I_\rho^{mso}\models Q_\phi(0)$, it follows that $\rho,0\models\phi$.
\begin{itemize}
% \item 
% If $\phi$ is a propositional atom $p$, then $\mathsf{t}(\phi,x)=p(x)$. Since $\mathsf{t}(\phi)$ holds at each point $x$ of $\mathcal{I}_\rho^{mso}$, we have that if $x\in p^\I$, then $\rho,x\models p$.
\item 
If $\phi =(\neg \theta_j$), then $\mathsf{t}(\phi,x) = (Q_{\phi}(x) \leftrightarrow (x \notin Q_{\theta_j}))$. Since $\mathsf{t}(\phi)$ holds
at every point $x$ of $\I_\rho^{mso}$, it holds that $x\in Q_{\phi}^\I$ iff $x\not\in Q_{\theta_j}^\I$. It follows by induction that $\rho,x\not\models \theta_j$. Thus, $\rho,x\models\phi$. 
\item
If $\phi = (\theta_j \wedge \theta_k)$, then $\mathsf{t}(\phi,x) = (Q_{\phi}(x) \leftrightarrow (Q_{\theta_j}(x) \wedge Q_{\theta_k}(x)))$. Since $\mathsf{t}(\phi)$ holds at every point $x$ of $\I_\rho^{mso}$, it follows that $x\in Q_{\phi}^\I$ iff $x\in Q_{\theta_j}^\I$ and $x\in Q_{\theta_k}^\I$. It follows by induction that $\rho,x\models\theta_j$ and $\rho,x\models\theta_k$. Thus, $\rho,x\models\phi$.
\item
If $\phi = (\theta_j \vee \theta_k)$, then $\mathsf{t}(\phi,x) = (Q_{\phi}(x) \leftrightarrow (Q_{\theta_j}(x) \vee Q_{\theta_k}(x)))$. Since $\mathsf{t}(\phi)$ holds at every point $x$ of $\I_\rho^{mso}$, it follows that $x\in Q_{\phi}^\I$ iff $x\in Q_{\theta_j}^\I$ or $x\in Q_{\theta_k}^\I$. It follows by induction that $\rho,x\models\theta_j$ or $\rho,x\models\theta_k$. Thus, $\rho,x\models\phi$.
\item
If $\phi = (X\theta_j)$, then $\mathsf{t}(\phi,x) = (Q_{\phi}(x)\leftrightarrow ((x \neq last)\wedge Q_{\theta_j}(x+1)))$.
Since $t(\phi)$ holds at every point $x$ of $\I_\rho^{mso}$, it follows that $x\in Q_{\phi}^\I$ iff $x\neq last$ and $x+1\in Q_{\theta_j}^\I$. It follows by induction that $x\neq last$ and $\rho,x\models\theta_j$. Thus, $\rho,x\models\phi$.
\item
If $\phi = (N\theta_j)$, then $\mathsf{t}(\phi,x) = (Q_{\phi}(x)\leftrightarrow ((x = last)\vee Q_{\theta_j}(x+1)))$. 
Since $\mathsf{t}(\phi)$ holds at every point $x$ of $\I_\rho^{mso}$, it follows that $x\in Q_{\phi}^\I$ iff $x=last$ or $x+1\in Q_{\theta_j}^\I$. It follows by induction that $x=last$ or $\rho,x\models\theta_j$. Thus, $\rho,x\models\phi$.

\item If $\phi = (\theta_j U \theta_k$), then $\mathsf{t}(\phi,x) = (Q_{\phi}(x) \leftrightarrow (Q_{\theta_k}(x) \vee ((x \neq last) \wedge Q_{\theta_j}(x) \wedge Q_{\phi}(x+1))))$. Since $\mathsf{t}(\phi)$ holds at every point $x$ of $\I_\rho^{mso}$, it follows that $x\in Q_{\phi}^\I$ iff $x \in Q^\I_{\theta_k}$ or $x \neq last \mbox{ with } x \in Q_{\theta_j} \mbox{ also }x+1\in Q_{\phi}^\I$. Thus, $\rho,x\models\phi$.

\item If $\phi = (\theta_j R \theta_k$), then $\mathsf{t}(\phi,x) = (Q_{\phi}(x) \leftrightarrow (Q_{\theta_k}(x) \wedge ((x = last) \vee Q_{\theta_j}(x) \vee Q_{\phi}(x+1))))$. Since $\mathsf{t}(\phi)$ holds at every point $x$ of $\I_\rho^{mso}$, it follows that $x\in Q_{\phi}^\I$ iff $x \in Q^\I_{\theta_k}$ with $x = last \mbox{ or } x \in Q_{\theta_j} \mbox{ or }x+1\in Q_{\phi}^\I$. Thus, $\rho,x\models\phi$.

\end{itemize}
\end{proof}

\subsection{Variations of \MSO Encoding}

\paragraph{\textbf{Constraint Form}} The following theorem guarantees the correctness of the \emph{Sloppy} variation.
\begin{thm}
Let $\phi$ be an \LTLf formula in \NNF, $\rho$ be a finite trace. Then $\rho \models \phi$ iff $\mathcal{I}_{\rho}^{mso} \models \mathsf{mso}_s(\phi)$.
\end{thm}

% The proof of Theorem~\ref{thm:msosloppy} is analogous to the proof of Theorem~\ref{thm:msofussy}. 
The crux of the proof here is that the $\leftrightarrow$ in $\mathsf{t}(\theta_i)$ is needed only to handle negation correctly. \emph{Sloppy} encoding, however, is applied only to \LTLf formulas in \NNF, so negation can be applied only to atomic propositions, which is handled by the base case $(\neg Q_p(x))$. In contrast, \BNF requires a general handling of negation, so \emph{Sloppy} cannot be applied to \LTLf formulas in \BNF.

\paragraph{\textbf{Variable Form}} The following lemma guarantees the correctness of the second-order terms introduced by the $\mathsf{lean}$ function.
\begin{lem}
Let $\phi$ be an \LTLf formula, $\rho$ be a finite trace. Then $\rho,x \models \theta_i$ iff $\mathsf{lean}(\theta_i)(x)$, where $x$ is the position in $\rho$.
\end{lem}
\begin{proof}
Suppose first that $\rho,x \models \theta_i$. We prove this inductively on the structure of $\theta_i$.
\begin{itemize}
\item If $\theta_i = \neg \theta_j$, then $\mathsf{lean}(\theta_i) = (\mathsf{ALIVE} \backslash \mathsf{lean}(\theta_j))$. $\mathsf{lean}(\theta_i)(x)$ holds since $\mathsf{lean}(\theta_i) = \{x~:~x \notin \mathsf{lean}(\theta_j)\}$ and $\mathsf{lean}(\theta_j) = \{x~:~\rho,x \models \theta_j\}$.

\item If $\theta_i = \theta_j \wedge \theta_k$, then $\mathsf{lean}(\theta_i) = (\mathsf{lean}(\theta_j)~\mbox{inter}~\mathsf{lean}(\theta_k))$. $\mathsf{lean}(\theta_i)(x)$ holds since $\mathsf{lean}(\theta_i) = \{x~:~x \in \mathsf{lean}(\theta_j) \mbox{ and } x \in \mathsf{lean}(\theta_k)\}$, $\mathsf{lean}(\theta_j) = \{x~:~\rho,x \models \theta_j\}$ and $\mathsf{lean}(\theta_k) = \{x~:~\rho,x \models \theta_k\}$.

\item If $\theta_i = \theta_j \vee \theta_k$, then $\mathsf{lean}(\theta_i) = (\mathsf{lean}(\theta_j)~\mbox{union}~\mathsf{lean}(\theta_k))$. $\mathsf{lean}(\theta_i)(x)$ holds since $\mathsf{lean}(\theta_i) = \{x~:~x \in \mathsf{lean}(\theta_j) \mbox{ or } x \in \mathsf{lean}(\theta_k)\}$, $\mathsf{lean}(\theta_j) = \{x~:~\rho,x \models \theta_j\}$ and $\mathsf{lean}(\theta_k) = \{x~:~\rho,x \models \theta_k\}$.

\item If $\theta_i = X\theta_j$, then $\mathsf{lean}(\theta_i) = ((\mathsf{lean}(\theta_j)-1) \backslash \{last\})$. $\mathsf{lean}(\theta_i)(x)$ holds since $\mathsf{lean}(\theta_i) = \{x~:~x \neq last \mbox{ and } x+1 \in \mathsf{lean}(\theta_j)\}$, $\mathsf{lean}(\theta_j) = \{x~:~\rho,x \models \theta_j\}$.

\item If $\theta_i = N\theta_j$, then $\mathsf{lean}(\theta_i) = ((\mathsf{lean}(\theta_j)-1)~\mbox{union}~\{last\})$. $\mathsf{lean}(\theta_i)(x)$ holds since $\mathsf{lean}(\theta_i) = \{x~:~x = last \mbox{ or } x+1 \in \mathsf{lean}(\theta_j)\}$, $\mathsf{lean}(\theta_j) = \{x~:~\rho,x \models \theta_j\}$.

\item If $\theta_i = \theta_j U \theta_k$ or $\theta_i = \theta_j R \theta_k$, then $\mathsf{lean}(\theta_i) = Q_{\theta_a}$. $\mathsf{lean}(\theta_i)(x)$ holds since $\mathsf{lean}(\theta_i)  = Q_{\theta_a} = \{x~:~\rho,x \models \theta_a\}$, where $Q_{\theta_a}$ is the corresponding second-order predicate for formula $\theta_i$.

\end{itemize}

Assume now that $\I_{\rho}^{mso} \models \mathsf{lean}(\theta_i)(x)$ with given interpretations of second-order predicates. We now prove $\rho,x \models \theta_i$ by induction over the structure on $\theta_i$.
\begin{itemize}
\item If $\theta_i = \neg \theta_j$, then $\mathsf{lean}(\theta_i) = (\mathsf{ALIVE} \backslash \mathsf{lean}(\theta_j))$. Since $\mathsf{lean}(\theta_i)(x)$ holds, we also have that $x \in \mathsf{lean}(\theta_i)$ iff $x \notin \mathsf{lean}(\theta_j)$. It follows by induction that $\rho,x \models \theta_i$.

\item If $\theta_i = \theta_j \wedge \theta_k$, then $\mathsf{lean}(\theta_i) = (\mathsf{lean}(\theta_j) ~\mbox{inter}~ \mathsf{lean}(\theta_k))$. Since $\mathsf{lean}(\theta_i)(x)$ holds, we also have that $x \in \mathsf{lean}(\theta_i)$ iff $x \in \mathsf{lean}(\theta_j)$ and $x \in \mathsf{lean}(\theta_k)$. It follows by induction that $\rho,x \models \theta_i$.

\item If $\theta_i = \theta_j \vee \theta_k$, then $\mathsf{lean}(\theta_i) = (\mathsf{lean}(\theta_j) ~\mbox{union}~ \mathsf{lean}(\theta_k))$. Since $\mathsf{lean}(\theta_i)(x)$ holds, we also have that $x \in \mathsf{lean}(\theta_i)$ iff $x \in \mathsf{lean}(\theta_j)$ or $x \in \mathsf{lean}(\theta_k)$. It follows by induction that $\rho,x \models \theta_i$.

\item If $\theta_i = X\theta_j$, then $\mathsf{lean}(\theta_i) = ((\mathsf{lean}(\theta_j)-1) \backslash \{last\})$. Since $\mathsf{lean}(\theta_i)(x)$ holds, we also have that $x \neq last \mbox{ and } x+1 \in \mathsf{lean}(\theta_j)\}$. It follows by induction that $\rho,x \models \theta_i$.

\item If $\theta_i = N\theta_j$, then $\mathsf{lean}(\theta_i) = ((\mathsf{lean}(\theta_j)-1) ~\mbox{union}~ \{last\})$. Since $\mathsf{lean}(\theta_i)(x)$ holds, we also have that $x = last \mbox{ or } x+1 \in \mathsf{lean}(\theta_j)\}$. It follows by induction that $\rho,x \models \theta_i$.

\item If $\theta_i = \theta_j U \theta_k$ or $\theta_i = \theta_j R \theta_k$, then $\mathsf{lean}(\theta_i) = Q_{\theta_a}$, where $Q_{\theta_a}$ is the corresponding second-order predicate. It follows by induction that $\rho,x \models \theta_i$.
\end{itemize}

\end{proof}

The following theorem guarantees the correctness of the \emph{Lean} variation.
\begin{thm1}
Let $\phi$ be an \LTLf formula, $\rho$ be a finite trace. Then $\rho \models \phi$ iff $\mathcal{I}_{\rho} \models \mathsf{mso}_\lambda(\phi)$.
\end{thm1}
\begin{proof}
If $\phi$ is a propositional atom $p$, then $\mathsf{mso}_\lambda(\phi)=Q_p(0)$. It is true that $\rho \models \phi$ iff $\I_\rho \models \mathsf{mso}_\lambda(\phi)$. If $\phi$ is an nonatomic formula, we prove this theorem in two directions.

Suppose first that $\rho$ satisfies $\phi$. We expand the monadic structure $\I_\rho$ with interpretations for $Q_{\theta_1}, Q_{\theta_2},\ldots,Q_{\theta_n}$ by setting $Q_{\theta_a}^\I = \{x~:~\rho,x \models \theta_a\}$. Let the expanded structure by $\I_\rho^{mso}$. By assumption, $\mathsf{lean}(\phi)(0)$ holds in $\I_\rho^{mso}$.
It remains to prove that $\I_\rho^{mso}\models(\forall x)(\bigwedge_{a=1}^{n}\mathsf{t}_\lambda(\theta_a,x))$, for each $U$ or $R$ subformula $\theta_a\in cl(\phi)$.
\begin{itemize}

\item If $\theta_a = (\theta_j U \theta_k)$, then $\mathsf{t}_\lambda(\theta_a,x) = (\mathsf{lean}(\theta_a)(x) \leftrightarrow (\mathsf{lean}(\theta_k)(x) \vee ((x \neq last) \wedge \mathsf{lean}(\theta_j)(x) \wedge \mathsf{lean}(\theta_a)(x+1))))$. This holds, since $\mathsf{lean}((\theta_j U \theta_k)) = \{x~:~\rho,x \models \theta_j U \theta_k\} = \{x~:~\rho,x \models \theta_k \mbox{ or } x \neq last \mbox{ with } \rho,x \models \theta_j \mbox{ also } \rho,x+1 \models \theta_a \}$, $\mathsf{lean}(\theta_j) = \{x~:~\rho,x \models \theta_j\}$, and $\mathsf{lean}(\theta_k) = \{x~:~\rho,x \models \theta_k\}$ with Lemma~\ref{lemma:lean};

\item If $\theta_a = (\theta_j R \theta_k)$, then $\mathsf{t}_\lambda(\theta_a,x) = (\mathsf{lean}(\theta_a)(x) \leftrightarrow (\mathsf{lean}(\theta_k)(x) \wedge ((x = last) \vee \mathsf{lean}(\theta_j)(x) \vee \mathsf{lean}(\theta_a)(x+1))))$. This holds, since $\mathsf{lean}((\theta_j R \theta_k)) = \{x~:~\rho,x \models \theta_j R \theta_k\} = \{x~:~\rho,x \models \theta_k \mbox{ with } x = last \mbox{ or } \rho,x \models \theta_j \mbox{ or } \rho,x+1 \models \theta_a \}$, $\mathsf{lean}(\theta_j) = \{x~:~\rho,x \models \theta_j\}$, and $\mathsf{lean}(\theta_k) = \{x~:~\rho,x \models \theta_k\}$ with Lemma~\ref{lemma:lean}.
\end{itemize}
%With above, it has been proven that $\mathcal{I}_{\rho}^{mso} \models mso(\phi)$; 

Assume now that $\I_\rho\models \mathsf{mso}_\lambda(\phi)$. This means that there is an expansion of $\I_\rho$ with monadic interpretations $Q_{\theta_a}^\I$ for each element $\theta_a$ of U or R subformulas in $cl(\phi)$ such that this expanded structure $\I_\rho^{mso}\models (\mathsf{lean}(\phi)(0))\wedge ((\forall x)(\bigwedge_{a=1}^{n} \mathsf{t}_\lambda(\theta_a,x)))$. If $\phi$ is not an $R$ or $U$ subformula, then it has been proven by Lemma~\ref{lemma:lean} that if $x \in \mathsf{lean}(\phi)$, then $\rho,x\models\phi$. We now prove by induction on $\phi$ that if $x \in Q_{\theta_a}^\I$, then $\rho,x\models\phi$. Since $\I_\rho^{mso}\models (\mathsf{lean}(\phi)(0))$, it follows that $\rho,0\models\phi$. 
\begin{itemize}
\item
If $\phi= (\theta_j U \theta_k$), then $\mathsf{t}_\lambda(\phi,x) = (\mathsf{lean}(\phi)(x) \leftrightarrow (\mathsf{lean}(\theta_k)(x) \vee ((x \neq last) \wedge \mathsf{lean}(\theta_j)(x) \wedge \mathsf{lean}(\phi)(x+1))))$. Since $\mathsf{t}_\lambda(\phi)$ holds at every point $x$ of $\I_\rho^{mso}$, it follows that $x\in \mathsf{lean}(\phi)$ iff $x \in \mathsf{lean}(\theta_k)$ or $x \neq last \mbox{ with } x \in \mathsf{lean}(\theta_j) \mbox{ also }x+1\in \mathsf{lean}(\phi)$. Moreover, $\mathsf{lean}(\phi) = Q_{\theta_a}$, where $Q_{\theta_a}$ is the corresponding second-order predicate. Thus, by induction hypothesis $\rho,x\models\phi$.
\item
If $\phi= (\theta_j R \theta_k$), then $\mathsf{t}_\lambda(\phi,x) = (\mathsf{lean}(\phi)(x) \leftrightarrow (\mathsf{lean}(\theta_k)(x) \wedge ((x = last) \vee \mathsf{lean}(\theta_j)(x) \vee \mathsf{lean}(\phi)(x+1))))$. Since $\mathsf{t}_\lambda(\phi)$ holds at every point $x$ of $\I_\rho^{mso}$, it follows that $x\in \mathsf{lean}(\phi)$ iff $x \in \mathsf{lean}(\theta_k)$ with $x = last \mbox{ or } x \in \mathsf{lean}(\theta_j) \mbox{ or }x+1\in \mathsf{lean}(\phi)$. Moreover, $\mathsf{lean}(\phi) = Q_{\theta_a}$, where $Q_{\theta_a}$ is the corresponding second-order predicate.  Thus, by induction hypothesis $\rho,x\models\phi$.

\end{itemize}
\end{proof}

\section{Compact \MSO Encoding}
The section gives more details about the Compact \MSO encoding described in Section~\ref{sec:omso}.
\subsection{\LTLf to \pltlf}

We define $\rho^R = \rho[|\rho|-1],\rho[|\rho|-2],\ldots,\rho[1],\rho[0]$ to be the reverse of $\rho$. Moreover, given language $\L$, we denote the reverse of $\mathcal{L}$ by $\mathcal{L}^R$ such that $\mathcal{L}^R$ collects all reversed sequences in $\mathcal{L}$. Formally speaking, $\mathcal{L}^R = \{\rho^R ~:~ \rho \in \mathcal{L}\}$.
The following theorem shows that \PLTLf formula $\phi^R$ accepts exactly the reversed language satisfying $\phi$.

% Here we show the omitted proof in the paper of the following theorem in Sec.~\ref{sec:omso}.
\begin{thm1}
Let $\mathcal{L}(\phi)$ be the language of $\phi$ and $\mathcal{L}^R(\phi)$ be the reversed language, then $\mathcal{L}(\phi^R) = \mathcal{L}^R(\phi)$.
\end{thm1}

\begin{proof}
$\mathcal{L}(\phi^R) = \mathcal{L}^R(\phi)$ iff for an arbitrary sequence $\rho \in \mathcal{L}(\phi)$ such that $\rho \models \phi$, it is true that $\rho^R \models \phi^R$. We prove the theorem by the induction over the structure of $\phi$. $last$ is used to denote the last instance such that $last = |\rho|-1$.
\begin{itemize}
\item Basically, if $\phi = p$ is an atom, then $\phi^R = p$, $\rho \models \phi$ iff $p\in\rho[0]$ such that $p \in \rho^R[last]$. Therefore, $\rho^R \models \phi^R$;

\item If $\phi = \neg \phi_1$, then $\phi^R = \neg \phi_1^R$, $\rho \models \neg \phi_1$ iff $\rho \nvDash \phi_1$, such that by induction hypothesis $\rho^R \nvDash \phi_1^R$ holds, therefore $\rho^R \models \phi^R$ is true;

\item If $\phi =\phi_1 \wedge \phi_2$, then $\phi^R = \phi_1^R \wedge \phi_2^R$, $\rho \models \phi$ iff $\rho$ satisfies both $\phi_1$ and $\phi_2$. By induction hypothesis $\rho^R \models \phi_1^R$ and $\rho^R \models \phi_2^R$ hold, therefore $\rho^R \models \phi^R$ is true;

\item If $\phi= X\phi_1$, $\phi^R = Y\phi_1^R$, $\rho \models \phi$ iff suffix $\rho'$ is sequence$\rho[1],\rho[2],\ldots,\rho[last]$ and $\rho' \models \phi_1$. By induction hypothesis, $\rho'^R \models \phi_1^R$ holds, in which case $\rho^R,{last-1} \models \phi_1^R$ is true, therefore $\rho^R \models \phi^R$ holds. 

\item If $\phi = \phi_1 U \phi_2$, $\rho \models \phi$ iff there exists $j$ such that $j~(0\leq j \leq last)$, suffix $\rho' = \rho[j],\rho[j+1],\ldots,\rho[last]$ satisfies $\phi_2$. Also for all $k$ such that $k~(0\leq k< j)$, $\rho'' = \rho[k],\rho[k+1],\ldots,\rho[last]$ satisfies $\phi_1$. By induction hypothesis, $\rho'^R \models \phi_1^R$ and $\rho''^R \models \phi_2^R$ hold, therefore we have $\rho^R,last-j \models \phi_2^R$ and $\forall k.last-j < k \leq last, \rho^R,k \models \phi_1^R$ hold such that $\rho^R \models \phi^R$. The proof is done.
\end{itemize}
\end{proof}

\subsection{\PLTLf to DFA}

Here we show the omitted proof in the paper of the following theorem that guarantees the correctness of \FOL encoding of \pltlf formula in Sec.~\ref{sec:omso}.

\begin{thm1}
Given a \PLTLf formula $\psi$, a finite trace $\rho$ and the corresponding interpretation $\mathcal{I}_{\rho}$ of $\rho$, $\rho \models \psi$ iff $\mathcal{I}_{\rho} \models \mathsf{fol_p}(\psi, last)$, $last = |\rho|-1$.
\end{thm1}

\begin{proof}
We prove the theorem by the induction over the structure of $\psi$.
\begin{itemize}
\item Basically, if $\psi = p$ is an atom, $\rho \models \psi$ iff $p\in\rho[last]$. By the definition of $\mathcal{I}$, we have that $last \in p^{\mathcal{I}_\rho}$. Therefore, $\rho \models \psi$ iff $\mathcal{I}_{\rho} \models \mathsf{fol_p}(p, last)$ holds;

\item If $\psi = \neg \psi$, $\rho \models \neg \psi$ iff $\rho \nvDash \psi$. By induction hypothesis it is true that $\mathcal{I}_{\rho} \nvDash \mathsf{fol_p}(\psi, last)$, therefore $\mathcal{I}_{\rho} \models \mathsf{fol_p}(\neg \psi, last)$ holds;

\item If $\psi =\psi_1 \wedge \psi_2$, $\rho \models \psi$ iff $\rho$ satisfies both $\psi_1$ and $\psi_2$. By induction hypothesis, it is true that $\mathcal{I}_{\rho} \models \mathsf{fol_p} (\psi_1,last)$ and $\mathcal{I}_{\rho} \models \mathsf{fol_p}(\psi_2, last)$. Therefore $\mathcal{I}_{\rho} \models \mathsf{fol_p}(\psi_1,last)\wedge \mathsf{fol_p}(\psi_2, last)$ holds;

\item If $\psi= Y\psi_1$, $\rho \models \psi$ iff prefix $\rho'= \rho[0],\rho[1],\ldots,\rho[last-1]$ of $\rho$ satisfies $\rho' \models \psi_1$. Let $\mathcal{I}_{\rho}'$ be the corresponding interpretation of $\rho'$, thus for every atom $p \in \P$, $i\in p^{\mathcal{I}_{\rho}'}$ iff $i\in p^{\mathcal{I}_{\rho}}$. By induction hypothesis it is true that $\mathcal{I}_{\rho}'\models \mathsf{fol_p} (\psi_1, last-1)$, therefore $\mathcal{I}_{\rho}\models \mathsf{fol_p} (Y\psi_1, last)$ holds. 

\item If $\psi = \psi_1 S \psi_2$, $\rho \models \psi$ iff there exists $j$ such that $0\leq j \leq last$ and prefix $\rho' = \rho[0],\rho[1],\ldots,\rho[j]$ of $\rho$ satisfies $\psi_2$ and for all $k$ such that $j< k \leq last$, $\rho'' = \rho[0],\rho[1],\ldots,\rho[k]$ satisfies $\psi_1$. Let $\mathcal{I}_{\rho}'$ and $\mathcal{I}_{\rho}''$ be the corresponding interpretations of $\rho'$ and $\rho''$. Thus for every atom $p \in \P$ it is true that 
$i\in p^{\mathcal{I}_{\rho}'}$ iff $i \in p^{\mathcal{I}_{\rho}}$, $i\in p^{\mathcal{I}_{\rho}''}$ iff $i \in p^{\mathcal{I}_{\rho}}$. By induction hypothesis it is true that $\mathcal{I}_{\rho}'\models \mathsf{fol_p} (\psi_2, last-j)$ and $\mathcal{I}_{\rho}''\models \mathsf{fol_p} (\psi_1, last-k)$ hold, therefore $\mathcal{I}_{\rho} \models \mathsf{fol_p}(\psi_1 S \psi_2,last)$. 
\end{itemize}
\end{proof}
